# Supplementary material for: Electron-lattice coupling contributions to polarization switching in charge-order-induced ferroelectrics
Source: arXiv:2103.16466 ancillary file (2022-02-18)
Supplement: Supplementary file 1 [file Supplementary_Materials.pdf]

# Supplementary Materials: Electron-lattice coupling contributions to polarization switching in charge-order-induced ferroelectrics

Yubo Qi, and Karin M. Rabe
*Department of Physics & Astronomy, Rutgers University, Piscataway, New Jersey 08854, United States*
(Dated: December 11, 2021)

## I. METHODS

All the first-principles density-functional-theory (DFT) calculations are performed with the generalized gradient approximation plus $U$ (GGA $+U$) method using the QUANTUM–ESPRESSO package [S1]. The on-site Coulomb interaction [S2] term $U$ and its rotationally invariant form $J$ are used with $U = 4$ eV and $J = 0.6$ eV for the vanadium $d$ orbitals and $U = 11$ eV and $J = 0.68$ eV for the La $f$ orbitals [S3–S7]. A 4×4×4 Monkhorst–Pack $k$-point mesh is used to sample the Brillouin zone [S8]. For simulating $(SrVO_3)_1(LaVO_3)_1$ superlattice structure, a $\sqrt{2}\times\sqrt{2}\times 2$ supercell (containing 20 atoms) is used. The plane-wave cutoff energy is 50 Ry. The force threshold for structural relaxation is $5.0\times10^{-6}$ Hartree per Bohr. The ferroelectric polarization is calculated using the Berry phase method with a 4×4×7 $k$-point grid [S9]. The up- and down-CO states are computed by setting the initial orbital occupations with the 'starting_ns_eigenvalue' command in the QUANTUM–ESPRESSO package.

To generate the electronic energy landscapes at different $R$ values in the plane of $Q_{OD}(\mathrm{V}_1)$ and $Q_{OD}(\mathrm{V}_2)$ [S10, S11], we begin with an artificial $(SrVO_3)_1(LaVO_3)_1$ superlattice structure with $R = 1$, and then gradually change $R$ to $R_0$, which is the value of the optimized structure. For each $R$ value, we generate various structures with different $Q_{OD}(\mathrm{V}_1)$ and $Q_{OD}(\mathrm{V}_2)$. Holding fixed the values of these lattice distortion amplitudes $[R,\ Q_{OD}(\mathrm{V}_1)$ and $Q_{OD}(\mathrm{V}_2)]$, we optimize each generated structure with two different initial electronic states, with $\mathrm{V}_1,\mathrm{V}_2 = \mathrm{V}^{3+},\mathrm{V}^{4+}$ and $\mathrm{V}_1,\mathrm{V}_2 = \mathrm{V}^{4+},\mathrm{V}^{3+}$ respectively. The computed energies corresponding to the two oppositely-polarized CO states are marked as $E_1$ and $E_2$, and their minimum $E\,[R, Q_{OD}(\mathrm{V}_1), Q_{OD}(\mathrm{V}_2)] = \min(E_1, E_2)$ is defined as the energy corresponding to the lattice modes $R, Q_{OD}(\mathrm{V}_1), Q_{OD}(\mathrm{V}_2)$ and used to construct the energy surface.

The $R$ value can be fixed by freezing the $z$ component of oxygen atoms connecting the oxygen octahedra along the $z$ direction. The $Q_{OD}(\mathrm{V}_i)$ value can be fixed by the $z$ component of the atom $\mathrm{V}_i$.

We also investigate the structural and CO-state changes under an electric field. We begin with the optimized down-polarization structure (in which $\mathrm{V}_1,\mathrm{V}_2 = \mathrm{V}^{3+},\mathrm{V}^{4+}$). An up-directed applied electric field, which is simulated with the method in Ref. [S12], is increased from 0 with 1.8 MV/cm as a step. At each step, the structure is optimized, and both the computed lattice and electronic structures and are used as the starting condition of the next step. And for each optimized structure, the competing electronically up-polarized CO state is also computed as a comparison.

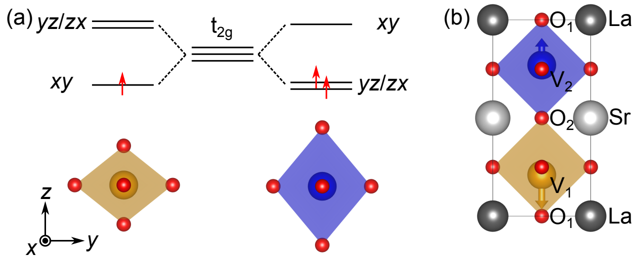


FIG. S1. (a) Schematic plot showing the orbital occupations in $\mathrm{V}^{3+}$ and $\mathrm{V}^{4+}$. (b) Schematic plot showing the structure of the $(SrVO_3)_1(LaVO_3)_1$ superlattice.

## II. DISPLACEMENTS IN THE SUPERLATTICE

In the $(SrVO_3)_1(LaVO_3)_1$ superlattice structure, the two V atoms are displaced antiparallel, pointing from the SrO layer to the LaO layer (the oxygen atoms in the SrO layer and LaO layer are denoted by $O_2$ and $O_1$ respectively, as shown in Fig. S1 (b)). Generally, the elongating of a chemical bond has to be compensated by the shortening of another chemical bond, and vice versa. Compared with Sr, La has a smaller ionic radius. As a result, in the $(SrVO_3)_1(LaVO_3)_1$ superlattice structure, the $LaO_1$ layers are tensilely strained. The La-$O_1$ bonds are elongated. Therefore, the V-$O_1$ bonds prefer to be shortened. Similarly, the the $SrO_2$ layers are compressively strained, Sr-$O_2$ bonds are shortened, and the V-$O_2$ bonds prefer to be elongated. As a result, the V atoms displace away from the the $SrO_2$ layer and toward the $LaO_1$ layer.

## III. OCCUPATION MATRICES

In this section, we list the occupation matrices of the majority spin electrons in $\mathrm{V}_1$ and $\mathrm{V}_2$ atoms in the $(SrVO_3)_1(LaVO_3)_1$ superlattice with $R = 1$. We find that charge disproportionation is still energetically favorable. For $\mathrm{V}_1$, the $d_{xy}$ orbital is mostly occupied, indicating a $\mathrm{V}^{4+}$ valence state [Fig. S1 (a)]. For $\mathrm{V}_2$, the $d_{zx}$ and $d_{zy}$ orbitals are mostly occupied, indicating a $\mathrm{V}^{3+}$ valence state [Fig. S1 (a)].

Occupation matrix of $V_1$

$$
\begin{array}{c}
 \\ d_{z^2} \\ d_{zx} \\ d_{zy} \\ d_{x^2-y^2} \\ d_{xy}
\end{array}
\begin{array}{c}
\begin{array}{ccccc} d_{z^2} & d_{zx} & d_{zy} & d_{x^2-y^2} & d_{xy} \end{array} \\
\begin{pmatrix}
0.345 & 0.005 & -0.004 & 0.003 & -0.026 \\
0.005 & 0.250 & 0.001 & -0.011 & 0.088 \\
-0.004 & 0.001 & 0.252 & 0.011 & -0.097 \\
0.003 & -0.011 & 0.011 & 0.303 & -0.082 \\
-0.026 & 0.088 & -0.097 & -0.082 & \boxed{0.911}
\end{pmatrix}
\end{array}
$$

Occupation matrix of $V_2$

$$
\begin{array}{c}
 \\ d_{z^2} \\ d_{zx} \\ d_{zy} \\ d_{x^2-y^2} \\ d_{xy}
\end{array}
\begin{array}{c}
\begin{array}{ccccc} d_{z^2} & d_{zx} & d_{zy} & d_{x^2-y^2} & d_{xy} \end{array} \\
\begin{pmatrix}
0.293 & 0.130 & -0.091 & -0.012 & 0.102 \\
0.130 & \boxed{0.787} & 0.104 & -0.066 & 0.183 \\
-0.091 & 0.104 & \boxed{0.757} & -0.022 & -0.253 \\
-0.012 & -0.066 & -0.022 & 0.276 & 0.007 \\
0.102 & 0.183 & -0.253 & 0.007 & 0.296
\end{pmatrix}
\end{array}
$$

The boxed numbers indicate the orbitals which are mostly occupied.

## IV. LATTICE CONSTANTS AND ATOMIC POSITIONS

### A. The $(SrVO_3)_1(LaVO_3)_1$ superlattice

The $(SrVO_3)_1(LaVO_3)_1$ superlattice has multiple competing low-energy charge-ordering structures, and can adopt a layered charge ordering (LCO) one with non-zero polarization [S7]. In the work, we focus on this LCO structure only, whose lattice parameters and atomic coordinates are shown in Table S1. The superlattice has a $a^-a^-c^+$ rotation pattern. As a result, the primitive cell is a $\sqrt{2} \times \sqrt{2} \times 2$ supercell containing 20 atoms.

### B. The $LuFe_2O_4$ primitive cell

The lattice parameters and atomic coordinates in a $LuFe_2O_4$ primitive cell was taken from Ref. [S13] Supplementary Materials Table 1. The structure is shown in Fig. S2.

### C. The $Fe_3O_4$ primitive cell

The lattice parameters and atomic coordinates in a $Fe_3O_4$ primitive cell was taken from Ref. [S14]. The charge ordering arrangements of the Fe ions are shown in Fig. S3.


[S1] P. Giannozzi, S. Baroni, N. Bonini, M. Calandra, R. Car, C. Cavazzoni, D. Ceresoli, G. L. Chiarotti, M. Cococcioni, I. Dabo, A. D. Corso, S. de Gironcoli, S. Fabris, G. Fratesi, R. Gebauer, U. Gerstmann, C. Gougoussis, A. Kokalj, M. Lazzeri, L. Martin-Samos, N. Marzari, F. Mauri, R. Mazzarello, S. Paolini, A. Pasquarello, L. Paulatto, C. Sbraccia, S. Scandolo, G. Sclauzero, A. P. Seitsonen, A. Smogunov, P. Umari, and R. M. Wentzcovitch, J. Phys.: Condens. Matter **21**, 395502 (2009).

[S2] A. Liechtenstein, V. I. Anisimov, and J. Zaanen, Phys. Rev. B **52**, R5467 (1995).

[S3] H. Sawada, N. Hamada, K. Terakura, and T. Asada, Phys. Rev. B **53**, 12742 (1996).

[S4] Z. Fang, N. Nagaosa, and K. Terakura, Phys. Rev. B **67**, 035101 (2003).

[S5] S. Biermann, A. Poteryaev, A. Lichtenstein, and A. Georges, Phys. Rev. Lett. **94**, 026404 (2005).

[S6] M. Czyżyk and G. Sawatzky, Phys. Rev. B **49**, 14211 (1994).

[S7] S. Y. Park, A. Kumar, and K. M. Rabe, Phys. Rev. Lett. **118**, 087602 (2017).

[S8] H. J. Monkhorst and J. D. Pack, Phys. Rev. B **13**, 5188 (1976).

[S9] R. D. King-Smith and D. Vanderbilt, Phys. Rev. B **47**, 1651 (1993).


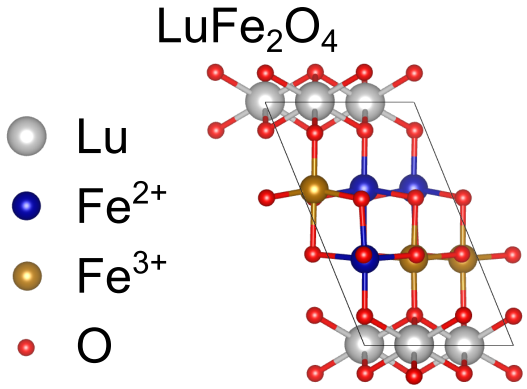


FIG. S2. The structure of $LuFe_2O_4$ primitive cell.


[S10] Q. Han and A. Millis, Phys. Rev. Lett. **121**, 067601 (2018).

[S11] A. B. Georgescu, O. E. Peil, A. S. Disa, A. Georges, and A. J. Millis, Proc. Natl. Acad. Sci. **116**, 14434 (2019).

[S12] I. Souza, J. Íniguez, and D. Vanderbilt, Phys. Rev. Lett. **89**, 117602 (2002).

[S13] H. J. Xiang, E. J. Kan, S.-H. Wei, M.-H. Whangbo, and J. Yang, Phys. Rev. B **80**, 132408 (2009).

[S14] E. J. W. Verwey, Nature **144**, 327 (1939).

| | $x$ | $y$ | $z$ |
|---|---|---|---|
| **a** | 3.92086 | -3.92085 | -0.00004 |
| **b** | 3.89192 | 3.89189 | 0.00542 |
| **c** | 0.00593 | 0.00582 | 7.71647 |
| V | 0.50040 | -0.00017 | 0.99347 |
| V | 0.49953 | 0.00123 | 0.50243 |
| V | 0.00047 | 0.50123 | 0.50243 |
| V | -0.00040 | 0.49983 | 0.99347 |
| O | 0.22833 | 0.22800 | 0.97377 |
| O | 0.76734 | 0.76773 | 0.04034 |
| O | 0.27168 | 0.72800 | 0.97378 |
| O | 0.73266 | 0.26772 | 0.04033 |
| O | 0.43996 | 0.99528 | 0.24001 |
| O | 0.06004 | 0.49526 | 0.24001 |
| O | 0.23361 | 0.23393 | 0.52733 |
| O | 0.76427 | 0.76564 | 0.46160 |
| O | 0.26639 | 0.73393 | 0.52732 |
| O | 0.73573 | 0.26564 | 0.46161 |
| O | 0.56048 | 0.00631 | 0.76263 |
| O | 0.93952 | 0.50633 | 0.76263 |
| La | 0.99838 | 0.01692 | 0.24954 |
| La | 0.50162 | 0.51692 | 0.24954 |
| Sr | 0.00958 | 0.98514 | 0.74889 |
| Sr | 0.49041 | 0.48514 | 0.74889 |

TABLE S1. lattice parameters and atomic coordinates in the $(SrVO_3)_1(LaVO_3)_1$ superlattice.

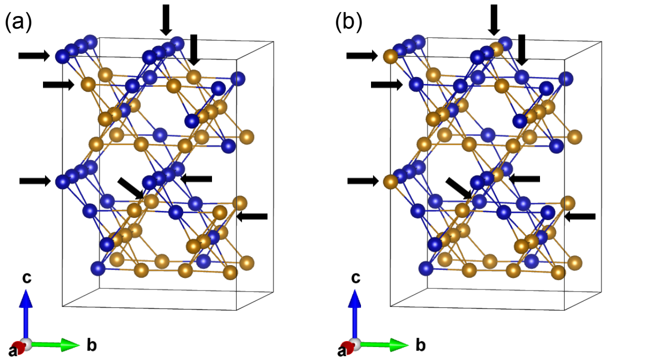


FIG. S3. CO patterns ($Fe^2+$ and $Fe^3+$ arrangement) of the $Fe_3O_4$ structure (a) before and (b) after the switching of valences of the Fe ions with similar $Q_{PB}$ values. The blue and orange spheres correspond to the $Fe^2+$ ion and $Fe^3+$ ion respectively. The ions which change their valence states are indicated by arrows.
